# Supplementary material for: Deterministic Function Computation with Chemical Reaction Networks
Source: arXiv:1204.4176 source file (2013-01-10)
Supplement: Supplementary file 1 [file appendix.tex]

\section{Technical Appendix}

\proofTechnicalLemmas
